# Supplementary material for: AmazonQA: A Review-Based Question Answering Task
Source: arXiv:1908.04364 source file (2019-08-20)
Supplement: Supplementary file 1 [file appendix.tex]

\appendix

\section{Hyperparameters}

\begin{table}[h]
    \centering
    \begin{tabular}{l|c} 
        \toprule
        \multicolumn{1}{c|}{Parameter} & \multicolumn{1}{c}{Value} \\ \midrule
        Batch Size & 64 \\
        Vocab Size & 30000 \\ 
        Embedding Size & 128 \\
        Encoder and Decoder & 3 Bi LSTMs \\
        Hdim Answers & 128 \\
        Hdim Questions & 128 \\
        Hdim Reviews & 128 \\
        Optimizer & Adam \\
        Learning Rate & 0.01 \\
        Max Question Length & 50 \\
        Max Answer Length & 100 \\
        Max Review Length & 100 \\
        Max Output Len & 100 \\
        Dropout & 0.2 \\
        Max Global Norm & 5.0 \\
        No. of Reviews Selected & 5 \\
        Teacher Forcing Ratio & 1.0 \\
        \bottomrule
    \end{tabular}
    \caption{Hyperparameters for the sequence to sequence language model $P(\mathcal{A} | \mathcal{Q}, \mathcal{R})$ with best performance}
    \label{tab:LM-Hype}
\end{table}

\begin{table}[h]
    \centering
    \begin{tabular}{l|c} 
        \toprule
        \multicolumn{1}{c|}{Parameter} & \multicolumn{1}{c}{Value} \\ \midrule
        Batch Size & 100 \\
        Vocab Size & 50000 \\ 
        Glove Embedding Size & 300 \\
        Char-Level Encoding & 1 Bi GRU \\
        Passage, Question Encoding & 3 Bi GRUs \\
        Hidden Units & 75  \\
        Optimizer & AdaDelta \\
        Learning Rate & 0.5 \\
        Max Question Length & 50 \\
        Max Review Length & 500 \\
        Dropout & 0.3 \\
        \bottomrule
    \end{tabular}
    \caption{Hyperparameters for the R-Net Baseline with best performance}
    \label{tab:RNet-Hype}
\end{table}

\label{sec:appendix}
