# Supplementary material for: AmazonQA: A Review-Based Question Answering Task
Source: arXiv:1908.04364 source file (2019-08-20)
Supplement: Supplementary file 2 [file supplemental.tex]

\section{Supplemental Material}
\label{sec:supplemental}
